# Supplementary material for: Higher criticism for rare and weak non-proportional hazard deviations in survival analysis
Source: arXiv:2310.00554 source file (2025-10-27)
Supplement: Supplementary file 1 [file appendix.tex]

\section{Empirical Phase Transition}
In this appendix we explain how to evaluate the empirical phase transition depicted in Figures~\ref{fig:sim_dense} and \ref{fig:sim_sparse}.
\par
We assume a fixed sample size pair $(n,N)$ and vector of base rates $P=(P_1,\ldots,P_N)$. For a given statistic $T_{n,N}$ and level $0<\alpha<1$, we first use $m$ Monte-Carlo samples to determine the $1-\alpha$ empirical Monte-Carlo quantile of $T_{n,N}$ under $H_0^{(n)}$. We denote this quantile by $t_{1-\alpha,M}$. Next, we divide the box $[r_{\min}, r_{\max}] \times [\beta_{\min},\beta_{\max}]$ into a grid. We identifies each cell in this grid with a single point, say, the bottom-left corner of the cell. For each cell and its representative point, we simulate $m$ Monte-Carlo samples of $H_1^{(n)}$ and record the values of the statistic $T_{n,N}$ in each sample. Let $k(t_{s}|H_1)$ be the number of times $T_{n,N}$ exceeds $t_{s}$. We fix a small level $0<\delta$ and say that $k(t_s|H_1)$ is \emph{significant} at the level $\delta$ if 
\[
\Pr \left( \Bin(m,s) \geq k(t_s|H_1) \right) \leq \delta.
\]
For each value of $\beta$, we fit the logistic function 
\[
\sigma(r|\theta_0(\beta),\theta_1(\beta)) = \frac{1}{1+e^{-(\theta_1(\beta) r + \theta_0(\beta))}} 
\]
to the cells on the strip $\{(\beta,r),\,  \leq r \in [r_{\min},r_{\max}]\}$. The x-intercept $\theta_0(\beta)$ is defined as the \emph{phase transition} point of this strip. The empirical phase transition curve is defined as $\{ \theta_0(\beta),\, \beta \in [\beta_{\min}, \beta_{max}]$\}.
